# Supplementary material for: ANNEXE: Unified Analyzing, Answering, and Pixel Grounding for Egocentric Interaction
Source: arXiv:2504.01472 source file (2025-04-02)
Supplement: Supplementary file 1 [file X_suppl.tex]

\clearpage
\setcounter{page}{1}
\maketitlesupplementary
 % 将节编号格式设置为字母
\setcounter{section}{0} % 重新从 0 开始编号

\begin{figure}[H]
	\centering
	\includegraphics[width=\linewidth]{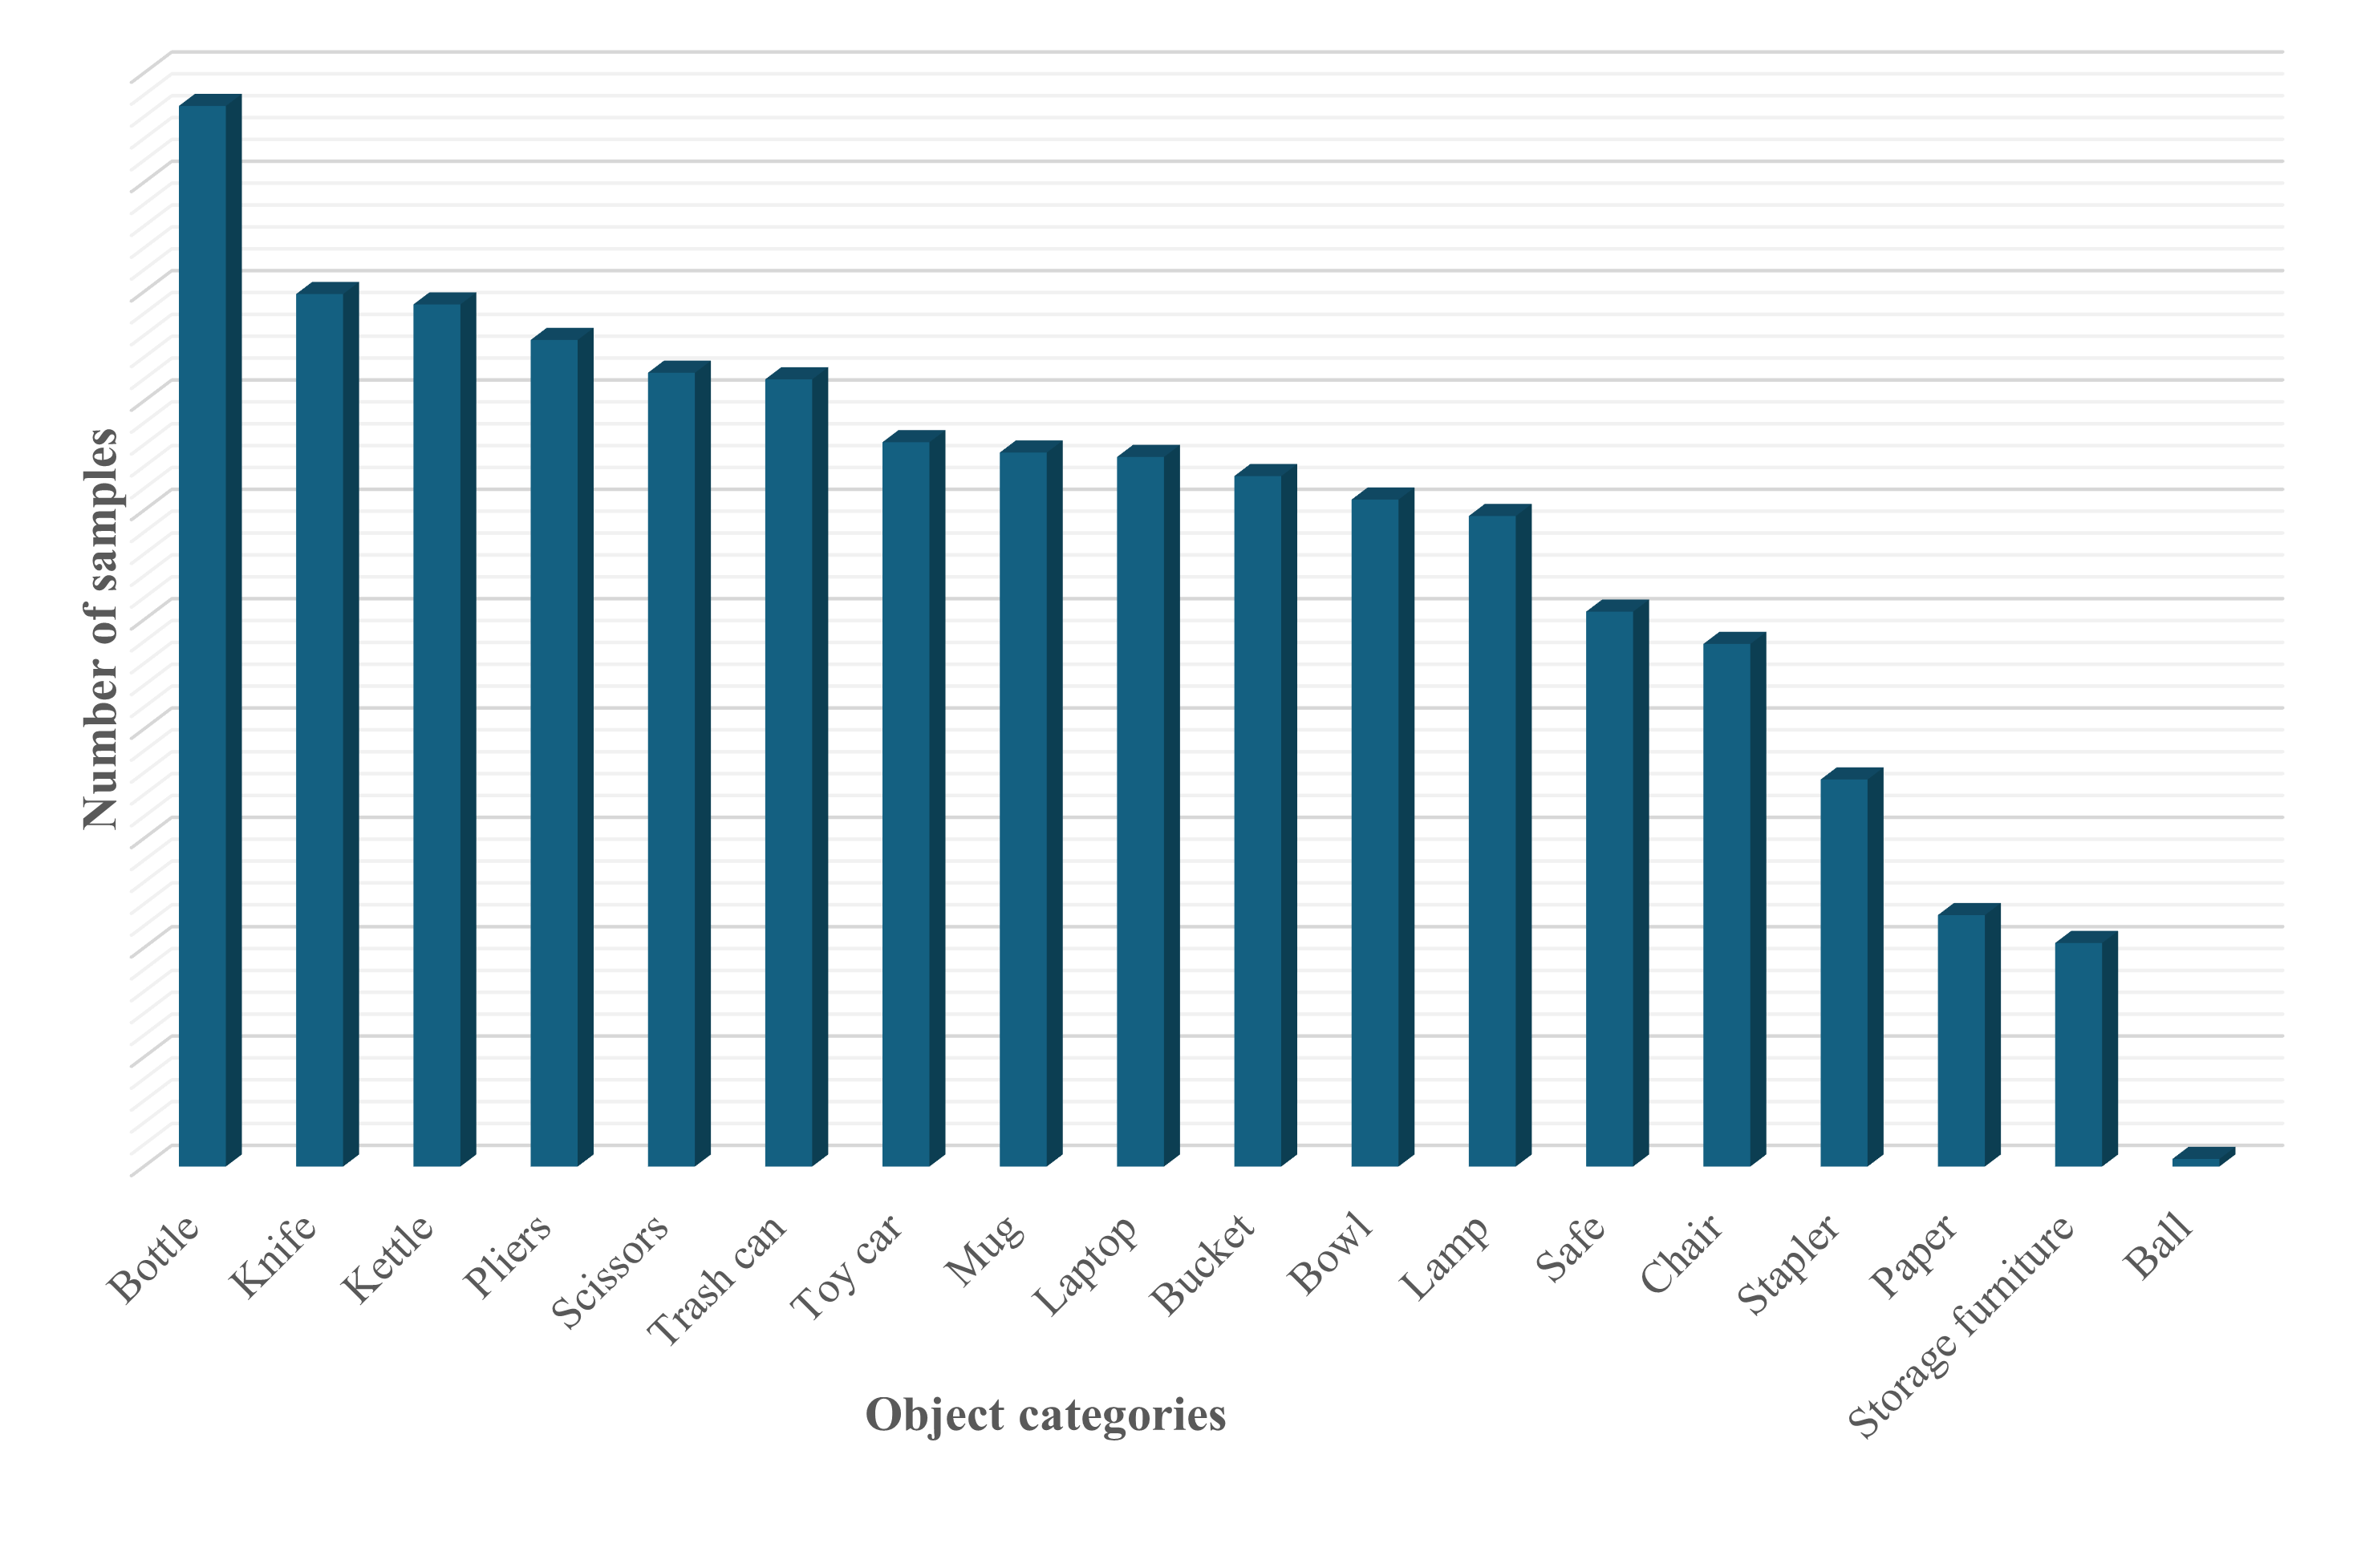}
	\caption{Distribution of interacting object categories in our Ego-IRGBench dataset.}
	\label{fig:supp:3}
\end{figure}

\begin{figure}[H]
	\centering
	\includegraphics[width=\linewidth]{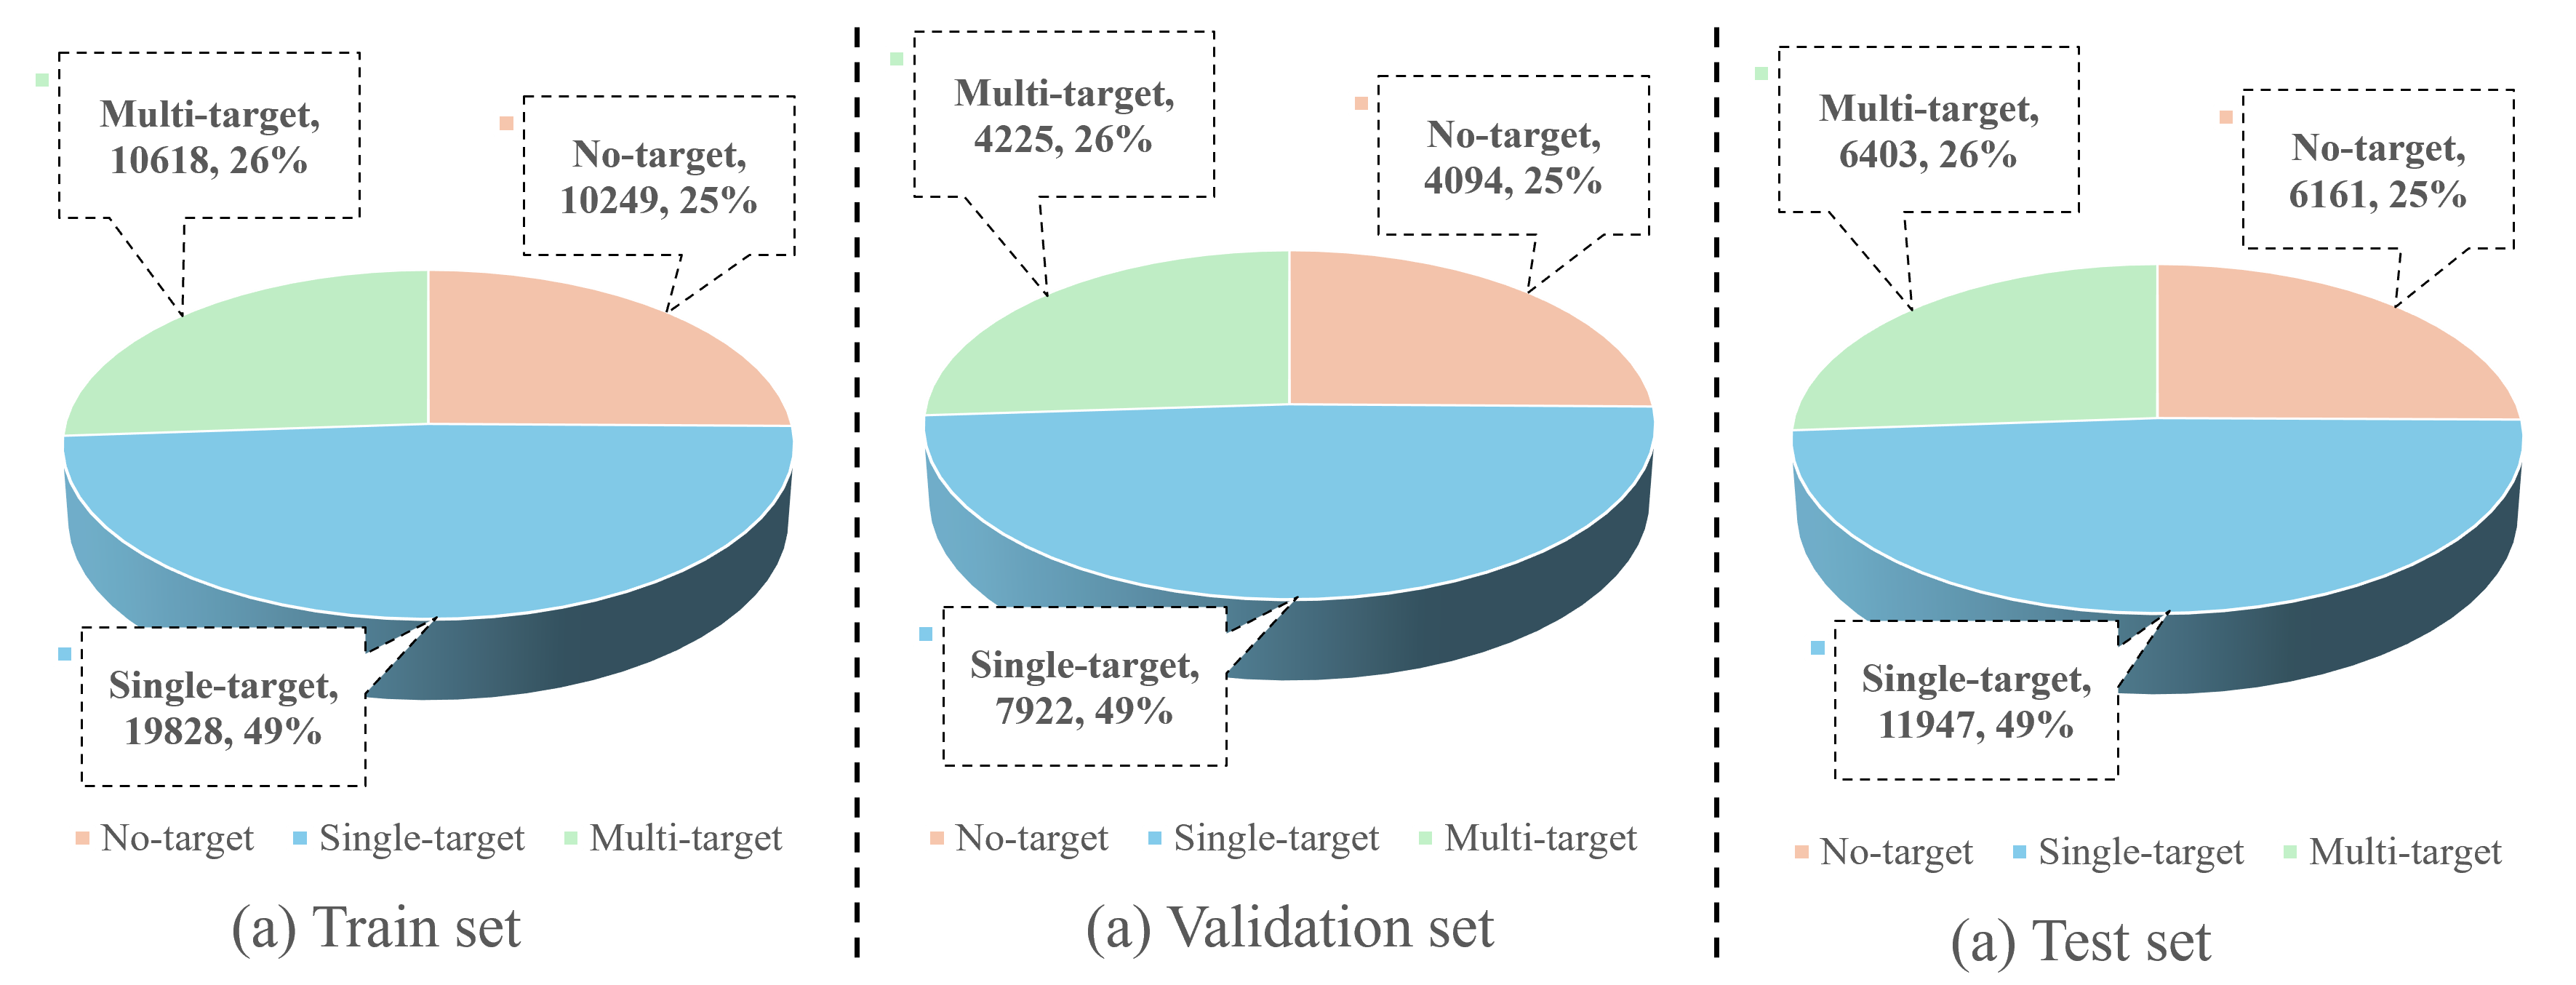}
	\caption{The proportion of single-target, multi-target, and no-target samples in the Ego-IRGBench training, validation, and test sets.}
	\label{fig:supp:4}
\end{figure}

\label{sec:supp:egointer}
\begin{figure*}[h]
	\centering
	\includegraphics[width=\textwidth]{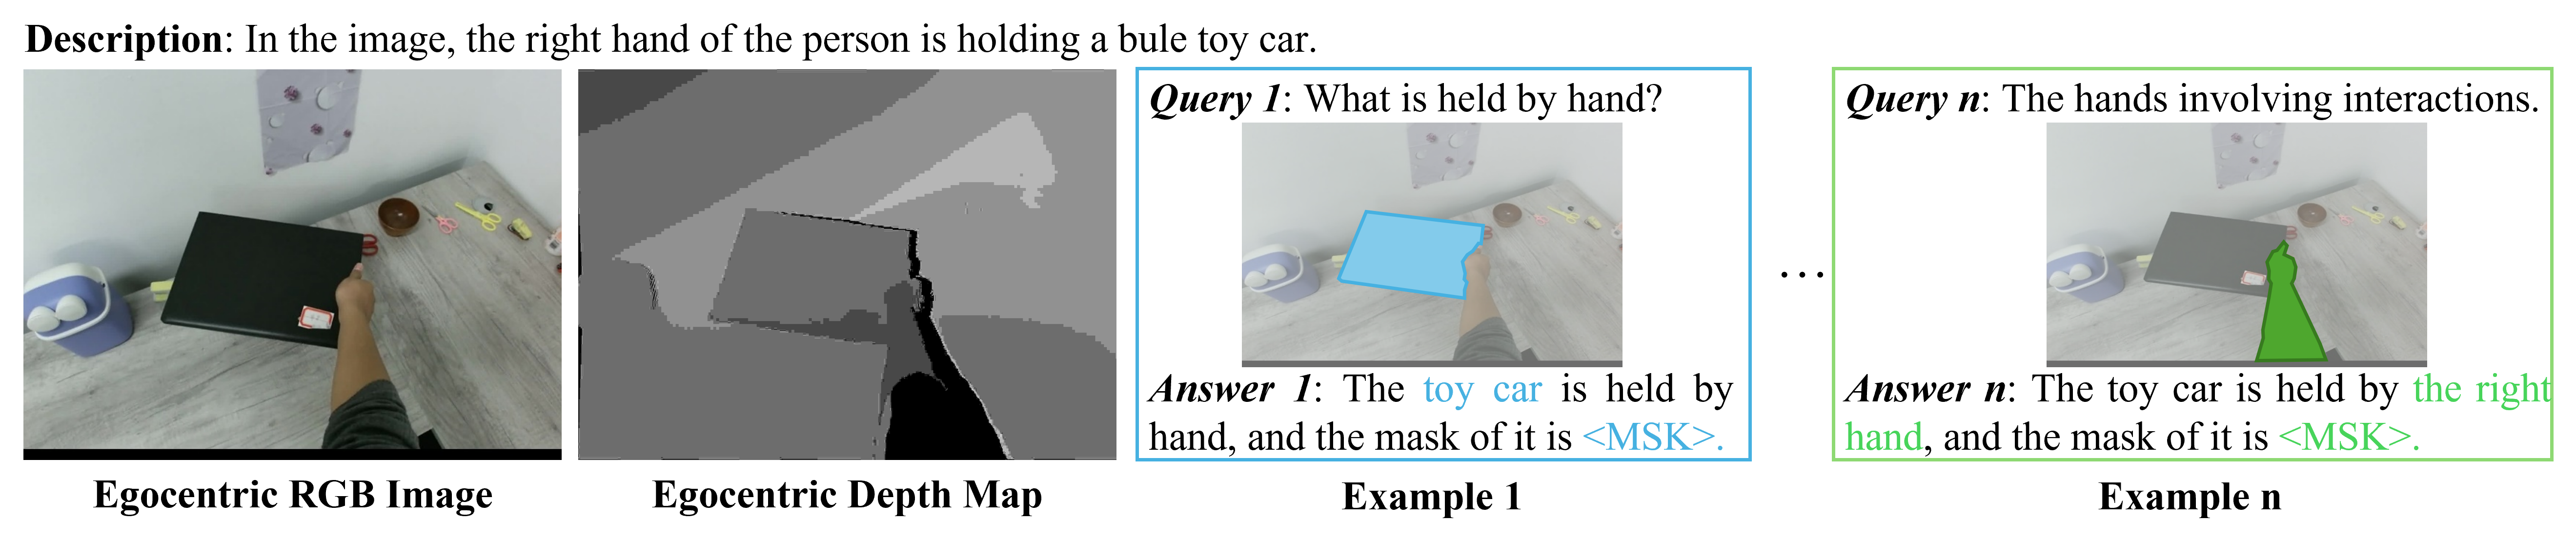}
	\caption{Structure of the Ego-IRGBench dataset. For each egocentric image, a depth map and query about interacting are provided. In addition, the query-answer-mask annotations are also included.}
	\label{fig:supp:1}
\end{figure*}

\begin{figure*}[h]
	\centering
	\includegraphics[width=\textwidth]{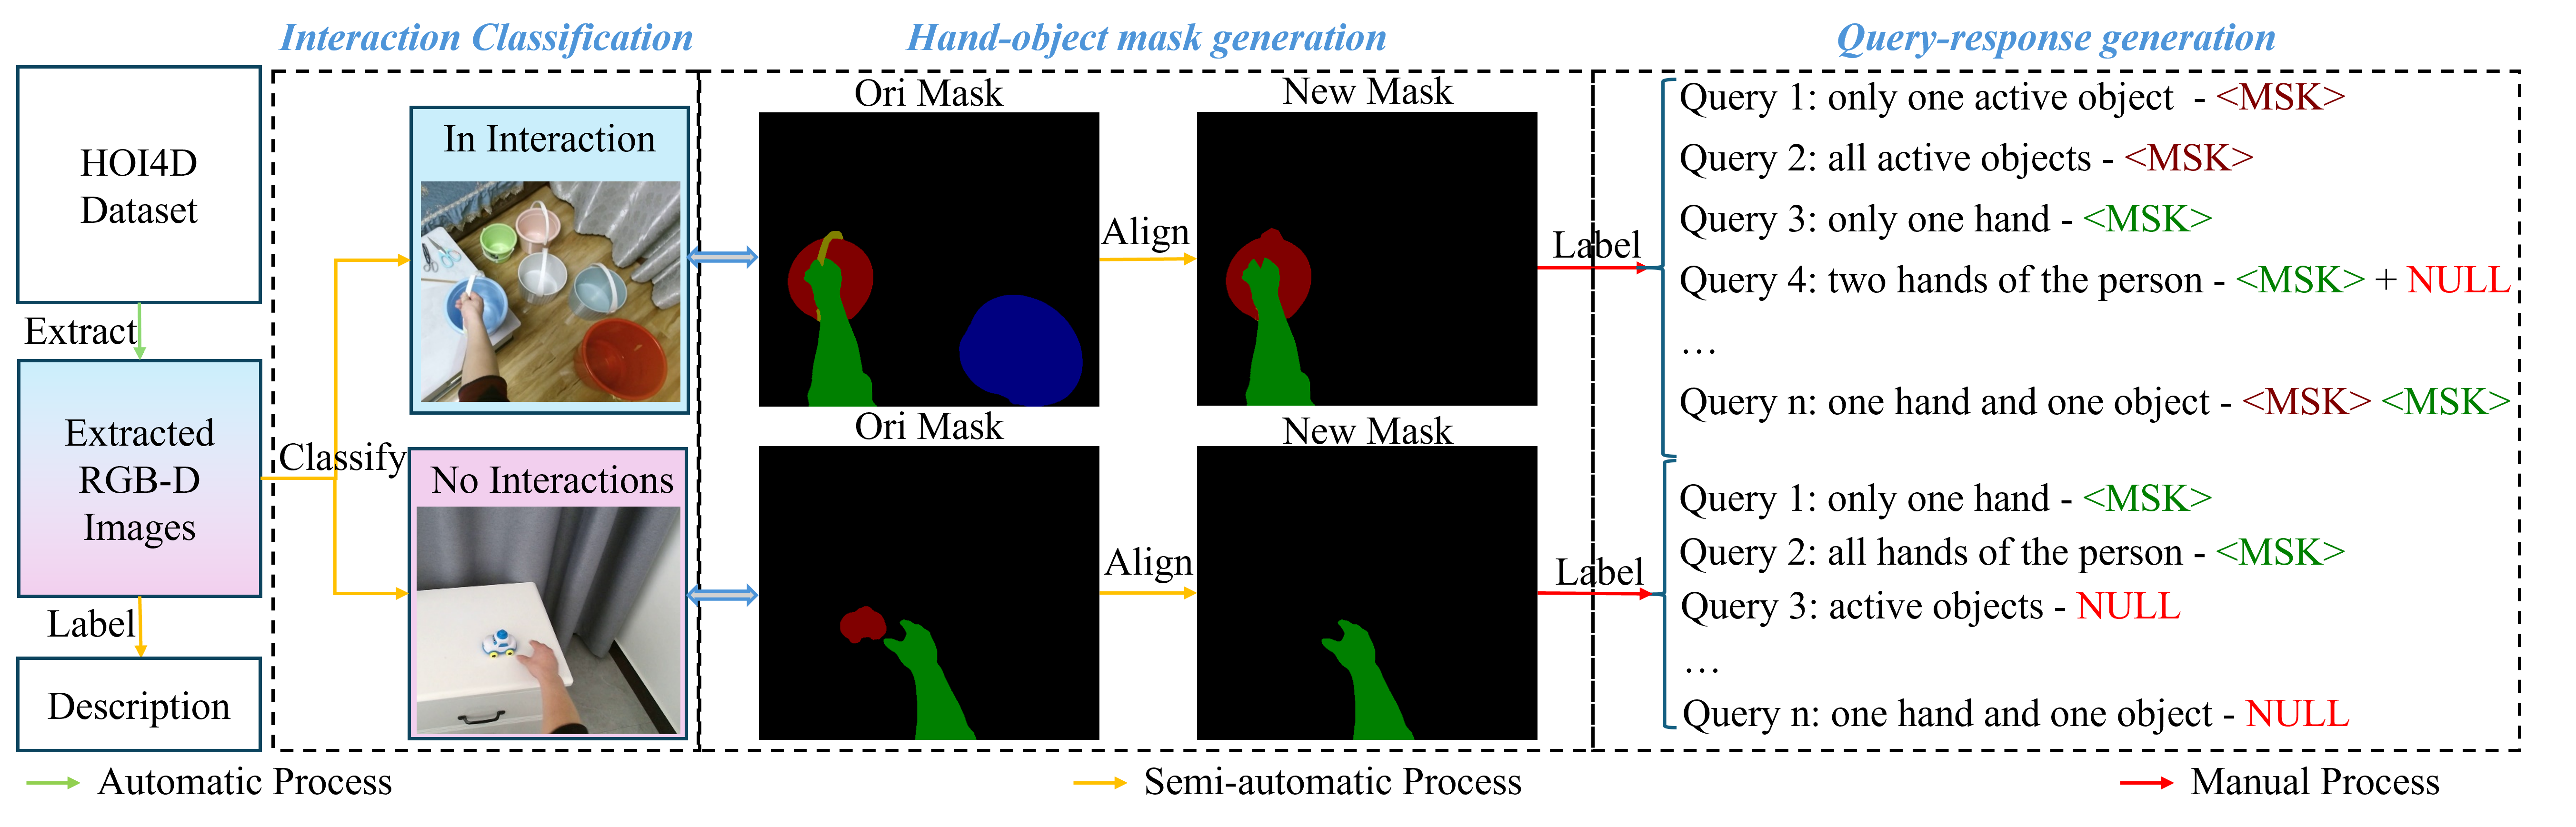}
	\caption{The overall pipeline to re-label the dataset with Ego-IRG annotations, which includes descriptions of interaction and corresponding query-answer-mask pairs.}
	\label{fig:supp:2}
    \vspace{-0.5cm}
\end{figure*}

\begin{figure*}[h]
	\centering
	\includegraphics[width=0.95\linewidth]{}
	\caption{Qualitative visualization results of our ANNEXE model on Ego-IRGBench validation and test sets.}
	\label{fig:supp:5}
\end{figure*}

\section{Ego-IRGBench}

\subsection{Structure and Scale}
\label{supp:dataset:scale}
In this paper, we create a large-scale dataset Ego-IRGBench for Ego-IRG (Egocentric reasoning and pixel grounding) task, which includes 20,681 RGB-D egocentric images and over 1.6 million queries about the interactions, along with corresponding textual and pixel-level responses. 
The structure of the dataset is shown in Fig. \ref{fig:supp:1}.

We also calculate the distribution of object categories in our dataset, which is shown in Fig. \ref{fig:supp:3}. 
We can observe that the Ego-IRGBench dataset includes 18 object categories. Some hard categories are also included with a limited number of samples, such as ``ball".
In addition, diverse queries for no-target, single-target, and multi-target are included in our Ego-IRGBench dataset. Thus, we count various types of queries on train, validation, and test sets, respectively, as depicted in Fig. \ref{fig:supp:4}.
We can observe that the proportion of different types of queries is basically consistent, which indicates the reasonableness of the dataset allocation.

\subsection{Step-wise Annotation Pipeline}
\label{supp:dataset:pipe}
To establish the Ego-IRGBench dataset, we employed experts to relabel the dataset based on the original HOI4D \cite{liu2022hoi4d} dataset. 
We developed an effective semi-automatic step-wise annotation pipeline to decrease the manual efforts consumed in building the dataset.
The pipeline is shown in Fig. \ref{fig:supp:2}.
The whole pipeline includes three essential steps: interaction classification, hand-object mask generation, and query-response generation.

\textbf{Step 1: interaction classification.}
The HOI4D \cite{liu2022hoi4d} dataset is a 4D egocentric dataset for category-level human-object interaction, which includes egocentric RGB-D videos and corresponding action categories, motion segmentation masks, 3D hand and object poses, object meshes, \emph{etc.}
Built upon the HOI4D \cite{liu2022hoi4d} dataset, we first extracted some RGB-D frames from egocentric videos with corresponding masks (original mask).
Furthermore, to establish the dataset quickly and efficiently, we adopt the interaction classification first, which is to classify the extracted RGB-D pairs into two categories: ``in interaction" and   ``without interactions."
For images where interaction occurs, we use a semi-manual approach to label the extracted frames with description annotations. Specifically, we manually labeled 400 images with descriptions of interactions between hands and objects. Then, we used these descriptions to fine-tune the multi-modal large language model to generate more descriptions. Finally, the generated descriptions are checked and modified by experts to be more diverse and comprehensive.
For images without interactions, we generated a description set including $\{$``The $<$left hand$>$ is not interacting with anything",  ``The person is hanging out the $<$hands$>$ without any interactions,"...$\}$. The final descriptions of these images are randomly selected from the description set.

\textbf{Step 2: hand-object mask generation.}
The extracted RGB-D egocentric frames are equipped with masks (original masks) in the HOI4D \cite{liu2022hoi4d} dataset. However, the original masks can not fulfill the requirements of our Ego-IRG task. Therefore, we asked the experts to align the original mask to generate the new mask manually.
Specifically, we set up five categories: left hand, right hand, objects interacting with the left hand, objects interacting with the right hand, and objects interacting with both hands. During the annotation process, we require that only masks of these five categories be saved or annotated, and other irrelevant categories in the original mask are deleted.

\textbf{Step 3: query-response generation.}
After generating the masks in step 2, we generated the query and corresponding textual and pixel-level responses manually.
Specifically, we disassemble and combine the masks annotated in the second step, annotate different queries and tokens according to different mask combinations, and obtain the corresponding query-token and mask pairs. The token is the basic component of the answer, which is the name of the objects that need to be segmented.
In addition, we used a template to generate the answers according to the mask and token.
The template we used is ``The mask of $<token_1>$ is $<MSK_1>$, the mask o  $<token_2>$ is $<MSK_2>$,..., and the mask of $<token_n>$ is $<MSK_n>$".
In this way, for each egocentric image, the query and corresponding text- and pixel-level responses are generated comprehensively.

\subsection{Criteria}
\label{supp:dataset:criteria}
To build up the benchmark for the Ego-IRG task, we set up the detailed evaluation criteria for three sub-tasks. 
Specifically, for the analyzing sub-task, which aims to generate the descriptions of interactions between hands and objects, we evaluate the quality of generated descriptions using METEOR \cite{banerjee2005meteor} and CIDEr \cite{vedantam2015cider} metrics.
Also, these two metrics are used to evaluate the answering sub-task, which aims to answer the query in textual response.
%To compute the METEOR between generated text $\textbf{T}_G$ and reference ground truth text $\textbf{T}_R$, the first step is to segment the $\textbf{T}_G$ and $\textbf{T}_R$ into words. 
%And stemming and synonym matching are applied to enhance matching between generated words and reference words, which can obtain the number of matching words $N_m$.
%\begin{align}
%    P = N_m / N_G, //
%    R = N_m / N_R, //
%    F_1 = 2 \times (P\times R)/(P+R), //
%    METEOR = F_1 \times (1-\alpha),
%\end{align}
In addition, we use cIoU \cite{lai2024lisa} to verify the accuracy of generated masks according to queries regarding interactions.

\subsection{Experimental Results}
\label{supp:exper}
We visualize some of the experimental results of our ANNEXE in this section, the results of which are shown in Fig. \ref{fig:supp:5}.
The results of the multi-target samples are shown in the first to third rows, and the results of single-target and no-target samples are exhibited in the fourth and fifth rows.
We can observe that the model can generate fluent and accurate descriptions for each egocentric image, which is similar to the description of ground truth (GT). The predicted answers for the query are also coherent and natural, along with precise pixel-level mask responses for queries regarding interactions.

% % 
% To split the supplementary pages from the main paper, you can use \href{https://support.apple.com/en-ca/guide/preview/prvw11793/mac#:~:text=Delete%20a%20page%20from%20a,or%20choose%20Edit%20%3E%20Delete).}{Preview (on macOS)}, \href{https://www.adobe.com/acrobat/how-to/delete-pages-from-pdf.html#:~:text=Choose%20%E2%80%9CTools%E2%80%9D%20%3E%20%E2%80%9COrganize,or%20pages%20from%20the%20file.}{Adobe Acrobat} (on all OSs), as well as \href{https://superuser.com/questions/517986/is-it-possible-to-delete-some-pages-of-a-pdf-document}{command line tools}.
